# Supplementary material for: Conformalization of Sparse Generalized Linear Models
Source: arXiv:2307.05109 source file (2023-07-11)
Supplement: Supplementary file 1 [file anotherappendix.tex]

\section{Whole Path Error Analysis}
\begin{theorem}
 The error between our estimate $\hat{\beta}(z')$ and the true weights $\beta(z')$ is upper bounded by 
 $$\left\|\hat{\beta}(z') - \beta(z')\right\|_2 \leq \left\|\mathcal{O}(\epsilon_{\text{tol}}) + \mathcal{O}(\epsilon_{\text{tol}} (z' - z_t)) +  \left[\int_{\bar{z}}^{z'} \frac{\partial \beta(z_t)}{\partial z} - \frac{\partial \beta(z^*)}{\partial z}dz^* \right]  + \frac{|A| L_3 M }{2} (\bar{z} - z_t)^2 \right\|_2 \text{.}$$
 Here, $\bar{z}$ is the point at where the active set changes after $z_t$ and follows the bound 

 $$\mathbb{E}(z' - \bar{z}) \leq \max\left(\underset{j\in A(z_t)^C}{\max} \frac{ X_j^\top \partial_{2} g(z_t) \pm \lambda}{ C\|X_j\|_2},  \underset{j\in A(z_t)}{\max} \frac{|A(z_t)|}{2} \cdot \beta_j(z_t)\right) - \min\left(\frac{ \lambda -  X_j\partial_2g(z_t) }{\|X_j\| L_3}, \frac{ -\lambda -  X_j\partial_2g(z_t) }{\|X_j\| L_3}\right)\text{.}$$
\end{theorem}
\begin{proof}
    The goal of this proof is to analyze the error at point $z'$ between our approximate homotopy and the true homotopy, $\|\hat{\beta}(z') - \beta(z')\|_2$. 
    We will use the definition from our algorithm that $$\hat{\beta}(z') = \hat{\beta}(z_t) + \frac{\partial \hat{\beta}(z_t)}{\partial z} (z' - z_t)\text{.}$$  Here, $z_t$ is the last point at which we ran our primal corrector. 
    Using this, we can decompose the error as the follows:
    \begin{align}
        \left\|\hat{\beta}(z') - \beta(z')\right\|_2 &= \left\|\hat{\beta}(z_t) + \frac{\partial \hat{\beta}(z_t)}{\partial z} (z' - z_t) - \beta(z') \right\|_2\\
        &= \left\|\hat{\beta}(z_t) + \frac{\partial \hat{\beta}(z_t)}{\partial z} (z' - z_t) - \beta(z') + \beta(z_t) - \beta(z_t) \right\|_2\\
        &=  \left\|\hat{\beta}(z_t) + \frac{\partial \hat{\beta}(z_t)}{\partial z} (z' - z_t) - \beta(z') + \beta(z_t) - \beta(z_t) \right\|_2\\
        &= \left\|\hat{\beta}(z_t) - \beta(z_t) + \frac{\partial \hat{\beta}(z_t)}{\partial z} (z' - z_t) - \left[\int_{z_t}^{z'} \frac{\partial \beta(z^*)}{\partial z} dz^*\right] \right\|_2\\
        &= \left\|\hat{\beta}(z_t) - \beta(z_t) + \left(\frac{\partial \hat{\beta}(z_t)}{\partial z} - \frac{\partial \beta(z_t)}{\partial z}\right) (z' - z_t) + \frac{\partial \beta(z_t)}{\partial z} (z' - z_t) - \left[\int_{z_t}^{z'} \frac{\partial \beta(z^*)}{\partial z}dz^* \right] \right\|_2\\
        &\leq \left\|\mathcal{O}(\epsilon_{\text{tol}}) + \mathcal{O}(\epsilon_{\text{tol}} (z' - z_t)) + \frac{\partial \beta(z_t)}{\partial z} (z' - z_t) - \left[\int_{z_t}^{z'} \frac{\partial \beta(z^*)}{\partial z}dz^* \right] \right\|_2\\
        &\leq \left\|\mathcal{O}(\epsilon_{\text{tol}}) + \mathcal{O}(\epsilon_{\text{tol}} (z' - z_t)) +  \left[\int_{z_t}^{z'} \frac{\partial \beta(z_t)}{\partial z} - \frac{\partial \beta(z^*)}{\partial z}dz^* \right] \right\|_2\\
        &\leq \left\|\mathcal{O}(\epsilon_{\text{tol}}) + \mathcal{O}(\epsilon_{\text{tol}} (z' - z_t)) +  \left[\int_{z_t}^{z'} \frac{\partial \beta(z_t)}{\partial z} - \frac{\partial \beta(z^*)}{\partial z}dz^* \right] \right\|_2\\
        &\leq \left\|\mathcal{O}(\epsilon_{\text{tol}}) + \mathcal{O}(\epsilon_{\text{tol}} (z' - z_t)) +  \left[\int_{z_t}^{z'} \frac{\partial \beta(z_t)}{\partial z} - \frac{\partial \beta(z^*)}{\partial z}dz^* \right] \right\|_2 \label{eq:beforesplit}
    \end{align}
    Therefore, we need to bound the rightmost term. We will split this integral into two parts: from $z_t to \bar{z}$ and from $\bar{z}$ to $z'$. $\bar{z}$ is where the active set changes. From $z_t$ to $\bar{z}$, the active set remains constant. We can upper bound the value from \Cref{eq:beforesplit} with this intuition as in  
    \begin{align}
        \mathcal{O}(\epsilon_{\text{tol}}) + \mathcal{O}&(\epsilon_{\text{tol}} (z' - z_t)) +  \left[\int_{z_t}^{z'} \frac{\partial \beta(z_t)}{\partial z} - \frac{\partial \beta(z^*)}{\partial z}dz^* \right]  \\
        &\leq  \left\|\mathcal{O}(\epsilon_{\text{tol}}) + \mathcal{O}(\epsilon_{\text{tol}} (z' - z_t)) +  \left[\int_{\bar{z}}^{z'} \frac{\partial \beta(z_t)}{\partial z} - \frac{\partial \beta(z^*)}{\partial z}dz^* \right]  + \left[\int_{z_t}^{\bar{z}} \frac{\partial \beta(z_t)}{\partial z} - \frac{\partial \beta(z^*)}{\partial z}dz^* \right] \right\|_2 \\
        &\leq \left\|\mathcal{O}(\epsilon_{\text{tol}}) + \mathcal{O}(\epsilon_{\text{tol}} (z' - z_t)) +  \left[\int_{\bar{z}}^{z'} \frac{\partial \beta(z_t)}{\partial z} - \frac{\partial \beta(z^*)}{\partial z}dz^* \right]  + \frac{|A| L_3 M }{2} (\bar{z} - z_t)^2 \right\|_2        
    \end{align}
    By \Cref{lem:overshoot},we have $\bar{z} - z' \leq \max\left(\underset{j\in A(z)^C}{\max} \frac{ X_j^\top \partial_{2} g(z) \pm \lambda}{ C\|X_j\|_2},  \underset{j\in A(z)}{\max} \frac{|A(z)|}{2} \cdot \beta_j(z_t)\right) - \min\left(\frac{ \lambda -  X_j\partial_2g(z_t) }{\|X_j\| L_3}, \frac{ -\lambda -  X_j\partial_2g(z_t) }{\|X_j\| L_3}\right)\text{.}$
\end{proof}

\begin{lemma}
\label{lem:overshoot}
Let $z^*$ be the where the active set truly changes after kink $z_t$. The difference between the $z_{t+1}$ the kink chosen by our algorithm and the true kink $z^*$ is upper bounded in expectation by 
$$\mathbb{E}(z^* - z_{t+1}) \leq \max\left(\underset{j\in A(z)^C}{\max} \frac{ X_j^\top \partial_{2} g(z) \pm \lambda}{ C\|X_j\|_2},  \underset{j\in A(z)}{\max} \frac{|A(z)|}{2} \cdot \beta_j(z_t)\right) - \min\left(\frac{ \lambda -  X_j\partial_2g(z_t) }{\|X_j\| L_3}, \frac{ -\lambda -  X_j\partial_2g(z_t) }{\|X_j\| L_3}\right) \text{.}$$
\end{lemma}
\begin{proof}
We first lower bound the value of $z^*$. There are two possible cases: $z^*$ is where a variable leaves the active set or when a variable joins the active set. We will look at the smallest possible $z^*$ achievable  by variable $j$ leaving or joining the active set, called the point $z_j^*$. In the first case, we require a variable $j$ in $A(z)$ to satisfy $\beta_j(z_j^*) = 0$ if $z_j^*$ is a kink. For this to hold, the value $\beta_j(z_t)$ has to move to $0$ as $z_t$ changes to $z_j^*$. To form an lower bound for $z_j^*$, we can use the upper bound of how fast $\beta_j(z_t)$ can decrease. Namely, we have $\frac{\partial \beta}{\partial z}(z") \leq \frac{\sigma_XL_2}{C}$ for any point $z"$.  Therefore, for some point $z_t - \epsilon$, the value of $|\beta_j(z_t - \epsilon)|$ satisfies $|\beta_j(z_t - \epsilon)| \geq |\beta_j(z_t)| - \epsilon \sigma_XC^{-1}L_2$. Therefore, to meet the condition of $\beta_j(z_t - \epsilon) = 0$, we need $\epsilon \leq \frac{|C\beta_j(z_t)|}{\sigma_X L_2}$. Therefore, $z_j^* \geq z_t - \frac{|\beta_j(z_t)|}{C^{-1}L_2}$.

For a variable joining the active set, we similarly desire to lower bound $z_j^*$ where $z_j^*$ satisfies, $\mathcal{I}_j(z_j^*) = 0$. This entails that $|X_j\partial_2g(z_j^*)| - \lambda$. To get this in terms of $z_t$, we can do this
\begin{align}
    \pm \lambda &= X_j\partial_2g(z_j^*)\\
    &=  X_j\partial_2g(z_j^*) - X_j\partial_2g(z_t) + X_j\partial_2g(z_t)\\
    &\geq  L_3\|X_j\|\left(z_j^* - z_t\right) + X_j\partial_2g(z_t)
\end{align}
Given that the algorithm chooses the first kink such that $\mathcal{I}_j(z_j^*) = 0$ is met, we can bound   $$z_j^*  \leq z_t - \min\left\{\frac{ \lambda -  X_j\partial_2g(z_t) }{\|X_j\| L_3}, \frac{ -\lambda -  X_j\partial_2g(z_t) }{\|X_j\| L_3}\right \}\text{.}$$ 

Now that we know the minimum distance from the next kink from the current kink, we can bound how far our algorithm overshoots the kink. We first state the update rules for our algorithm. 
\paragraph{Lower bounding the overshoot}

For a variable $j$ leaving the active set, the potential next kink is 
$$\hat{z}_{t+1}^j = z_t + \frac{\beta_j(z_t)}{\left[\left(\frac{\partial H}{\partial \beta}\right)^{-1}\frac{\partial H}{\partial y}\frac{\partial y}{\partial z}\right]_j} \text{ or } -\infty\text{.}$$
Moreover, for a variable $j$ joining the active set, the potential next kink is 
$$\hat{z}_{t+1}^j = z +  \frac{-X_j \partial_2 g(z) \pm \lambda}{X_j\left[\partial_{2,1}g(z)^\top \frac{\partial y}{\partial{z}} + \partial_{2,2}g(z)^\top \frac{\partial \beta}{\partial z}\right]} \text{ or } -\infty\text{.}$$
To find our next kink, we look at the maximum of such possible values. 
We start by computing 
$$\underset{j \in A(z)^c}{\max} \hat{z}_{t+1}^j\text{.}$$
Here, we need to make an assumption on the distribution of the gradients. In the worst case, there do exist situations where gradients in the denominator are $0$ for all $j$, which causes the algorithm to select $\min(y)$ as the next kink. This, however, is extremely pessimistic. We state this assumption here
\begin{assumption}
    The gradient $\frac{\partial \beta_j}{\partial z}$ for each variable $j$ is a random variable obeying a uniform distribution on the range $[-L_2, L_2]$.
\end{assumption}
This is a strong assumption, but not unreasonable. Now, if the numerator and the denominator have the same sign, the kink found will be greater than the current kink, which violates the homotopy. Therefore, we need to estimate the number of variables where the numerator and denominator are of different signs. Given this uniform assumption, the number of variables in the active set that satisfy this condition is a random variable called $\mathcal{X}$ with the expected value $\mathbb{E}(\mathcal{X})= |A(z)^c|/2$ and variance $Var(\mathcal{X}) = |A(z)|/4$. 
Therefore, given $\alpha$ variables satisfy this condition, we can use the knowledge that the minimum order statistics of a set of $n$ uniform random variables on the interval $[0, 1]$ has expected value $\frac{1}{n+1}$ and variance $\frac{1}{n^2}$. Therefore, the minimum value of the gradient in this set is in expectation is   $\mathbb{E}\left(\underset{j \in A(z)}{\min} \frac{\partial \beta_j}{\partial z}\right) \geq \frac{2}{|A(z)|} $ in expectation over the uniform distribution of gradients. Combining this with the term above, we get the estimate of the kink seen by a variable $j$ leaving the active set is upper bounded 
$z_{t+1,j} \geq z_t - \frac{|A(z)|}{2} \cdot \max(\beta_j(z_t))$. We now look at the second case where a variable joins the active set. We will similarly try to lower bound the denominator. For all elements in the inactive set, $\frac{\partial \beta_j}{\partial z}(z_t) = 0$. Therefore, we have
\begin{align}
  X_j^\top\partial_{2,1} g(z)\frac{\partial y}{\partial z} + X_j^\top\partial_{2,2} g(z)\frac{\partial H}{\partial y}\frac{\partial y}{\partial z} &\geq  C\|X_j\|_2 \left(1 + \frac{\partial \beta_j}{\partial z} \right) \\
  &\geq C\|X_j\|_2
\end{align}
Therefore, the potential amount of overshoot of the value has the following bound 
$$\frac{X_j^\top \partial_{2} g(z) \pm \lambda}{X_j^\top\partial_{2,1} g(z)\frac{\partial y}{\partial z} + X_j^\top\partial_{2,2} g(z)\frac{\partial \beta}{\partial z}} \leq \frac{X_j^\top \partial_{2} g(z) \pm \lambda}{ C\|X_j\|_2} \text{.}$$
Therefore, $z_{t+1}$ is upper bounded by the minimum of these two overshoots.
$$z_{t+1} \geq z_t - \max\left(\underset{j\in A(z)^C}{\max} \frac{ X_j^\top \partial_{2} g(z) \pm \lambda}{ C\|X_j\|_2},  \underset{j\in A(z)}{\max} \frac{|A(z)|}{2} \cdot \beta_j(z_t)\right)\text{.}$$
\end{proof}

% \begin{proof}
%     Given that the overshoot occurs till a point $z^*$ when it should have stopped at $z_{t+1}$. At point $z_{t+1}$, the algorithms active set of variables will match the true set of active variables. Therfore, by Theorem 7.1, we know that the error at point $z_{t+1}$ is upper bounded by
%     $$\|\beta_A(z') - \hat{\beta}_A(z')\|_2 \leq \frac{|A|L_3M}{2}(z' - z)^2$$. After that point, we can only pessimistically bound the worst case deviatioin. That is, if $\frac{\partial \beta}{\partial z} $ is chosen for the linearization, the error from any point $z' \in [z^*, z_{t+1}$ incurs error at most
%     $$\|\beta_A(z') - \hat{\beta}_A(z')\|_2 \leq (z' - z_{t+1})(|L_2| + \|\frac{\partial \beta}{\partial z}\|_2) + \frac{|A|L_3M}{2}(z_{t+1} - z_t)^2$$ Such a bound is intuitive. The error is small while the algorithms active set is the same as the truth, but is heavily penalized when it overshoots the kink, or $z^* - z'$ is large. However, we have bounded the amount we can overshoot the kink above. 

% \end{proof}
